# Supplementary material for: Principal Component Flow Map Learning of PDEs from Incomplete, Limited, and Noisy Data
Source: arXiv:2407.10854 source file (2024-12-24)
Supplement: Supplementary file 1 [file appendix.tex]

and $$\mathbf{V}_n = \mathbf{V}_{n-1} + \varepsilon\left(\mathbf{V}_{n-1},\ldots,\mathbf{V}_{n-N_{mem}}\right).$$ The difference is $$\mathbf{V}_{n-1} - \Pi_{out}\Pi_{in}\bar{\mathbf{V}}_{n-1} + \varepsilon\left(\mathbf{V}_{n-1},\ldots,\mathbf{V}_{n-N_{mem}}\right) -  \Pi_{out}\mathbf{N}\left(\Pi_{in}\bar{\mathbf{V}}_{n-1},\ldots,\Pi_{in}\bar{\mathbf{V}}_{n-N_{mem}}\right)$$

\begin{align}
    e(t_n) &= \left\|\mathbf{V}_n-\bar{\mathbf{V}}_n\right\|_2\\
    &= \left\|\mathbf{V}_n-\left(\Pi_{out}\Pi_{in}\bar{\mathbf{V}}_{n-1}+\Pi_{out}\mathbf{N}\left(\Pi_{in}\bar{\mathbf{V}}_{n-1},\ldots,\Pi_{in}\bar{\mathbf{V}}_{n-N_{mem}}\right)\right)\right\|_2\\
    &= \left\|\mathbf{V}_n-\Pi_{out}\Pi_{in}\bar{\mathbf{V}}_{n-1}-\Pi_{out}\mathbf{N}\left(\Pi_{in}\bar{\mathbf{V}}_{n-1},\ldots,\Pi_{in}\bar{\mathbf{V}}_{n-N_{mem}}\right)\right\|_2\\
    &= \left\|\mathbf{V}_{n-1}+\varepsilon(\mathbf{V}_{n-1},\ldots,\mathbf{V}_{n-N_{mem}})-\Pi_{out}\Pi_{in}\bar{\mathbf{V}}_{n-1}-\Pi_{out}\mathbf{N}\left(\Pi_{in}\bar{\mathbf{V}}_{n-1},\ldots,\Pi_{in}\bar{\mathbf{V}}_{n-N_{mem}}\right)\right\|_2\\
    &= \left\|\mathbf{V}_{n-1}-\Pi_{out}\Pi_{in}\bar{\mathbf{V}}_{n-1}\right\|_2+\left\|\varepsilon(\mathbf{V}_{n-1},\ldots,\mathbf{V}_{n-N_{mem}})-\Pi_{out}\mathbf{N}\left(\Pi_{in}\bar{\mathbf{V}}_{n-1},\ldots,\Pi_{in}\bar{\mathbf{V}}_{n-N_{mem}}\right)\right\|_2\\
    &= \left\|\mathbf{V}_{n-1}-\Pi_{out}\Pi_{in}\mathbf{V}_{n-1}\right\|_2+\|\Pi_{out}\Pi_{in}\|_2e(t_{n-1})+\left\|\varepsilon(\mathbf{V}_{n-1},\ldots,\mathbf{V}_{n-N_{mem}})-\Pi_{out}\mathbf{N}\left(\Pi_{in}\bar{\mathbf{V}}_{n-1},\ldots,\Pi_{in}\bar{\mathbf{V}}_{n-N_{mem}}\right)\right\|_2\\
    &= \varepsilon^{proj}_{n-1}+\|\Pi_{out}\Pi_{in}\|_2e(t_{n-1})+\left\|\varepsilon(\mathbf{V}_{n-1},\ldots,\mathbf{V}_{n-N_{mem}})-\Pi_{out}\mathbf{N}\left(\Pi_{in}\bar{\mathbf{V}}_{n-1},\ldots,\Pi_{in}\bar{\mathbf{V}}_{n-N_{mem}}\right)\right\|_2\\
    &= \varepsilon^{proj}_{n-1}+\|\Pi_{out}\Pi_{in}\|_2e(t_{n-1})+\left\|\varepsilon(\mathbf{V}_{n-1},\ldots,\mathbf{V}_{n-N_{mem}})-\Pi_{out}\hat{\varepsilon}(\hat{\mathbf{V}}_{n-1},\ldots,\hat{\mathbf{V}}_{n-N_{mem}})\right\|_2 + \left\|\Pi_{out}\hat{\varepsilon}(\hat{\mathbf{V}}_{n-1},\ldots,\hat{\mathbf{V}}_{n-N_{mem}})-\Pi_{out}\mathbf{N}\left(\Pi_{in}\bar{\mathbf{V}}_{n-1},\ldots,\Pi_{in}\bar{\mathbf{V}}_{n-N_{mem}}\right)\right\|_2\\
    &= \varepsilon^{proj}_{n-1}+\|\Pi_{out}\Pi_{in}\|_2e(t_{n-1})+\left\|\varepsilon(\mathbf{V}_{n-1},\ldots,\mathbf{V}_{n-N_{mem}})-\Pi_{out}\hat{\varepsilon}(\hat{\mathbf{V}}_{n-1},\ldots,\hat{\mathbf{V}}_{n-N_{mem}})\right\|_2\\ &+ \left\|\Pi_{out}\right\|_2\left\|\hat{\varepsilon}-\mathbf{N}\right\|_2\left\|(\hat{\mathbf{V}}_{n-1},\ldots,\hat{\mathbf{V}}_{n-N_{mem}})-\left(\Pi_{in}\bar{\mathbf{V}}_{n-1},\ldots,\Pi_{in}\bar{\mathbf{V}}_{n-N_{mem}}\right)\right\|_2\\
    &= \varepsilon^{proj}_{n-1}+\|\Pi_{out}\Pi_{in}\|_2e(t_{n-1})\\
    &+\left\|\varepsilon(\mathbf{V}_{n-1},\ldots,\mathbf{V}_{n-N_{mem}})-\Pi_{out}\hat{\varepsilon}(\Pi_{in}\mathbf{V}_{n-1},\ldots,\Pi_{in}\mathbf{V}_{n-N_{mem}})\right\|_2\\ &+ \left\|\Pi_{out}\right\|_2\left\|\hat{\varepsilon}-\mathbf{N}\right\|_2\left\|\Pi_{in}\right\|_2\sum_{k=1}^{N_{mem}}e(t_{n-k})\\
    &= \varepsilon^{proj}_{n-1}+\left\|\Pi_{out}\Pi_{in}\right\|_2e(t_{n-1})+\varepsilon^{\Delta}_{n} + \left\|\Pi_{out}\right\|_2\left\|\hat{\varepsilon}-\mathbf{N}\right\|_2\left\|\Pi_{in}\right\|_2\sum_{k=1}^{N_{mem}}e(t_{n-k})
\end{align}
where the bar denotes approximation.

Assume
\begin{align}
    \dot{\v} &= A_{11}\v+A_{12}\w\\
    \dot{\w} &= A_{21}\v+A_{22}\w.
\end{align}
Mori-Zwanzig says
\begin{align}
    \frac{d\v}{dt}(t) &= A_{11}\v(t)+A_{12}\int_0^te^{A_{22}(t-s)} A_{21}\v(s)ds+A_{21}e^{A_{22}t}\w(0) \\
    V_r\frac{d\hat{\v}}{dt}(t) &= A_{11}V_r\hat{\v}(t)+A_{12}\int_0^te^{A_{22}(t-s)} A_{21}V_r\hat{\v}(s)ds+A_{21}e^{A_{22}t}\w(0)\\
    V_r^TV_r\frac{d\hat{\v}}{dt}(t) &= V_r^TA_{11}V_r\hat{\v}(t)+V_r^TA_{12}\int_0^te^{A_{22}(t-s)} A_{21}V_r\hat{\v}(s)ds+V_r^TA_{21}e^{A_{22}t}\w(0)\\
\end{align}
where $\v = C^T\hat{\v}$, implying
\begin{align}
    \dot{\v} &= V_r^TA_{11}V_r\v+V_r^TA_{12}\w\\
    \dot{\w} &= A_{21}\v+A_{22}\w.
\end{align}

interesting because we need reduced dynamics to exist on observable variables

$\x=U_r\Sigma_r V_r^T$ then $\x V_r = U_r\Sigma_r$

Then system is

If $A=U\Sigma V^T$ is an SVD of the dynamics, 

\begin{align}
    \dot{\v} &= U_{11}\Sigma_{11}V_{11}^T\v+U_{12}\Sigma_{12}V_{12}^T\w\\
    \dot{\w} &= U_{21}\Sigma_{21}V_{21}^T\v+U_{22}\Sigma_{22}V_{22}^T\w.
\end{align}

or

\begin{align}
    \dot{\u} = A\u = U\Sigma V^T\u
\end{align}
